# Supplementary material for: SemEval-2024 Task 9: BRAINTEASER: A Novel Task Defying Common Sense
Source: arXiv:2404.16068 source file (2024-04-22)
Supplement: Supplementary file 1 [file word_puzzle.tex]

\section{Word Puzzle Example}\label{ssec:word_example}

Table~\ref{tab:word_example} presents a word puzzle with its reconstruction examples

\begin{table*}[!t]
  \begin{center}
  \small
    \caption{Overview of a word puzzle example and its reconstruction versions.}
    
    \label{tab:word_example}
    % \resizebox{\textwidth}{!}{
    \begin{tabular}{ p{1.7cm} | p{6.4cm} | p{6.8cm} } 
     \hline
     {Adv Strategy} & {Question} &  {Answers} \\ 
     % \toprule
     \cline{1-3}
         \multirow{4}*{-}  &  & \textbf{The letter N.}   \\
         &  What part of London is in France? & The letter O.  \\
         &  & The letter L.    \\
         & & None of the above.  \\
    \hline 
         &  
         &\textbf{The letter N.}  \\
         Semantic Re- & Which area of London is inside France? &The letter O.\\
         construction &  & The letter L.   \\
         & & None of the above.  \\
    \hline 
          & 
         &\textbf{The letter A.}  \\
         Context Re- & What part of Korea is in China?&  The letter E.\\
         construction &  & The letter R.\\
         & & None of the above.  \\
    \hline 
    \end{tabular}
    % }
  \end{center}
\end{table*}
